# Supplementary material for: Multi-resolution filters for massive spatio-temporal data
Source: arXiv:1810.04200 ancillary file (2019-11-13)
Supplement: Supplementary file 1 [file supplement.pdf]

# Supplementary material to "Multi-resolution filters for massive spatio-temporal data"

Marcin Jurek* Matthias Katzfuss*†

## S1 Proof of the exactness of MRF when $r_0 = n_{\mathcal{G}}$

In this section, we discuss one of the settings mentioned in Section 4.1 under which Algorithm 2 (MRD) is exact. Because the only approximation made in Algorithm 1 is

$$\mathbf{\Sigma}_{t|t-1} \approx \mathbf{B}\mathbf{B}' \tag{S1}$$

where $\mathbf{B} = \text{MRD}(\mathbf{\Sigma}^F_{t|t-1})$, the MRF is exact whenever (S1) holds with equality. As stated in Section 4.1, this is the case when $M = 0$ and $r_0 = n_{\mathcal{G}}$. Then Algorithm 2 reduces to computing $\mathbf{W} = \mathbf{\Sigma}^F_{t|t-1}$ and $\mathbf{V} = \mathbf{\Sigma}^F_{t|t-1}$. Hence, we have

$$\mathbf{B} = \mathbf{B}^0 = \mathbf{W}\mathbf{V}^{-\frac{1}{2}}$$

and

$$\mathbf{\Sigma}_{t|t-1} = \mathbf{B}\mathbf{B}' = \mathbf{W}\mathbf{V}^{-\frac{1}{2}}\mathbf{V}^{-\frac{1}{2}}\mathbf{W}' = \mathbf{\Sigma}^F_{t|t-1}.$$

## S2 More on distributed computation

As discussed briefly in Section 4.3, the MRF algorithm is well suited to distributed computations. This can be achieved by extending the approach in Katzfuss (2017, Sect. 3.5), as outlined here. Let us consider a set up in which node $\mathcal{N}_{j_1,\ldots,j_m}$ only stores the submatrix $\mathbf{B}_{t|t}[\mathcal{I}_{j_1,\ldots,j_m}, \mathcal{K}_{j_1,\ldots,j_m}]$ and the mean vector $\boldsymbol{\mu}_{t|t}[\mathcal{I}_{j_1,\ldots,j_m}]$. In order to execute the forecast step, we need to multiply $\mathbf{B}_{t-1|t-1}$ and $\boldsymbol{\mu}_{t-1|t-1}$ by $\mathbf{A}_t[\,:\,, \mathcal{I}_{j_1,\ldots,j_m}]$. In general, information from other computational nodes might be needed for this operation, but in our case only a small amount of data is required, because we assumed $\mathbf{A}_t$ to be local (see Assumption 2). Similarly, the MRD decomposition can largely be performed locally as its main computational burden is in calculating the $\mathbf{W}^l_{j_1,\ldots,j_m}$ matrices.

In the update step, computing $\boldsymbol{\mu}_{t|t}$ is accomplished by a series of matrix-vector multiplications. Under Assumption 1, calculating $\mathbf{H}_t'\mathbf{R}_t^{-1}(\mathbf{y}_t - \mathbf{H}_t\boldsymbol{\mu}_{t|t-1})$ can be executed separately on each node, provided the corresponding blocks of the $\mathbf{H}_t$ and $\mathbf{R}_t$ matrices are sent to same

*Department of Statistics, Texas A&M University
†Corresponding author: katzfuss@gmail.com

node. In order to obtain the $\mathbf{B}_{t|t}$ matrix, we need the Cholesky factor of $\mathbf{\Lambda}$ and its product with $\mathbf{B}_{t|t-1}$. Computation of elements $\mathbf{L}_t[\mathcal{K}_{j_1,\ldots,j_m}, \mathcal{K}_{j_1,\ldots,j_k}]$, $m < k$, can be mostly handled by node $\mathcal{N}_{j_1,\ldots,j_m}$. Moreover, since it already holds the $\mathbf{B}_{t|t-1}[\mathcal{I}_{j_1,\ldots,j_m}, \mathcal{K}_{j_1,\ldots,j_m}]$ block, which it acquired in the forecast step, it can also be tasked with calculating the $\mathbf{B}_{t|t}[\mathcal{I}_{j_1,\ldots,j_m}, \mathcal{K}_{j_1,\ldots,j_m}]$ block, since that requires little communication with other nodes.

# S3 Connections to multi-resolution autoregressive models

The idea of the multi-resolution analysis of spatial stochastic processes has been explored in great depth (e.g., Chou et al., 1994a,b; Willsky, 2002; Frakt and Willsky, 2001; Ferreira and Lee, 2007; Choi et al., 2010), and gave rise to many fast algorithms in the field of signal processing (e.g., Chou et al., 1994a; Luettgen and Willsky, 1995). The general focus of this strand of literature was on scale-recursive state-space models on trees and using Kalman-filter-like inference to derive the distribution of variables corresponding to the nodes of the tree. Building on these developments for purely spatial domains, several authors (e.g., Huang et al., 2002; Johannesson et al., 2003; Tzeng et al., 2005) applied the multi-resolution paradigm in modelling spatio-temporal stochastic processes. These approaches can be expressed using a random-effects process with spatial basis functions that are either constant or step-wise.

In this section we show how the MRA, which powers the multi-resolution filter (see Section 5.2), can be described in these terms.

Definition S1. (Frakt and Willsky, 2001) *Let $\mathcal{S}(\mathcal{V}, E)$ be a directed acyclic graph. For a given node $v$, let $\gamma(v)$ denote the parent node of $v$ and let $x(v)$ be a random vector associated with $v$. Then $x(\cdot)$ is a zero-mean* multi-resolution autoregressive process *(MAR) if*

$$x(v) = A(v)x(\gamma(v)) + w(v), \tag{S2}$$

*where $w(v)$ is white, uncorrelated with $x(w)$ for any $w \in \mathcal{V}$ and has autocovariance $Q(v)$.*

To show that the MRA is a MAR, we start with the observation that if $\mathbf{\Sigma} \approx \mathbf{B}\mathbf{B}'$ and we take $\boldsymbol{\eta} \sim \mathcal{N}(\mathbf{0}, \mathbf{I})$, then for $\mathbf{x} := \mathbf{B}\boldsymbol{\eta}$ we have $\mathbf{x} \sim \mathcal{N}(\mathbf{0}, \mathbf{B}\mathbf{B}')$. Now let us partition the vector $\mathbf{x}$ into segments whose sizes correspond to those of blocks $\mathbf{B}^1, \ldots \mathbf{B}^M$. We can then write

$$\mathbf{x} = \mathbf{B}\boldsymbol{\eta} = \mathbf{B}^0\boldsymbol{\eta}^0 + \mathbf{B}^1\boldsymbol{\eta}^1 + \cdots + \mathbf{B}^M\boldsymbol{\eta}^M$$

and define the level-$m$ approximation as

$$\mathbf{x}^m = \mathbf{B}^0\boldsymbol{\eta}^0 + \cdots + \mathbf{B}^m\boldsymbol{\eta}^m.$$

In order to represent $\mathbf{x}$ in the MAR form, we also need to define the graph $\mathcal{F} = (\mathcal{V}, \mathcal{E})$ that will provide indexing for the elements of $\mathbf{x}$. Let

$$\mathcal{V} = \{v_0\} \cup \{v_1, \ldots, v_J\} \cup \{v_{11}, v_{12}, \ldots, v_{JJ}\} \cup \ldots \tag{S3}$$

be the set of vertices. We associate each vertex with some subdomain in the hierarchy described in Section 3.4.1. For example, $v_0$ and $v_{j_1,\ldots,j_m}$ would correspond to $\mathcal{D}$ and $\mathcal{D}_{j_1,\ldots,j_m}$,

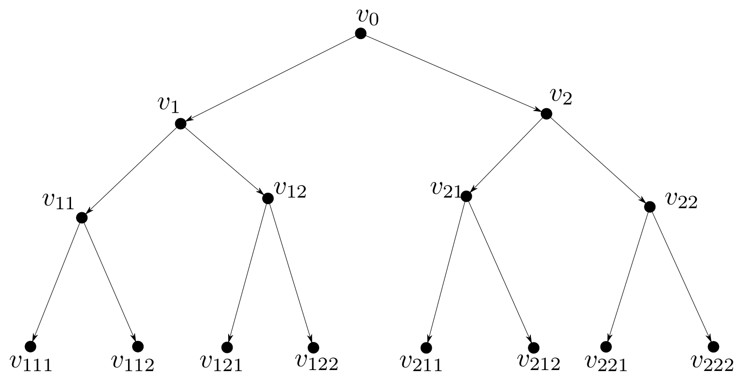


Figure S1: Graph $\mathcal{F}$ for $M = 3$, $J = 2$

respectively. Next, we define the set of edges $\mathcal{E}$ in a way that represents the domain partitioning hierarchy:

$$\mathcal{E} = \{v_0 \to v_j | j = 1, \dots J\} \cup \bigcup_{j=1}^{J} \{v_j \to v_{jk} | k = 1, \dots, J\} \cup \dots \tag{S4}$$

Figure S1 illustrates what this graph might look like.

We can now associate vertex $v_{j_1,\dots,j_m}$ with the $m$-th level approximation of the elements of vector $\mathbf{x}$ corresponding to grid points in $\mathcal{D}_{j_1,\dots,j_m}$. More precisely, using the notation of Definition S1, we can express it as

$$x(v_{j_1,\dots,j_m}) = \mathbf{B}^0 \boldsymbol{\eta}^0 + \mathbf{B}^1[\mathcal{I}_{j_1,\dots,j_m}, \mathcal{K}_{j_1}]\, \boldsymbol{\eta}^1 + \mathbf{B}^1[\mathcal{I}_{j_1,\dots,j_m}, \mathcal{K}_{j_1,j_2}]\, \boldsymbol{\eta}^2 + \dots + \mathbf{B}^m[\mathcal{I}_{j_1,\dots,j_m}, \mathcal{K}_{j_1,\dots,j_m}]\, \boldsymbol{\eta}^m.$$

This implies that the scale-recursive equations analogous to (S2) can then be written as

$$x(v_{j_1,\dots,j_m}) = \mathbf{I} \cdot x(v_{j_1,\dots,j_{m-1}}) + w(v_{j_1,\dots,j_m}),$$

where $w(v_{j_1,\dots,j_m}) = \mathbf{B}^m[\mathcal{I}_{j_1,\dots,j_m}, \mathcal{K}_{j_1,\dots,j_m}]\boldsymbol{\eta}^m$. From the definition of $\boldsymbol{\eta}$, it is clear that $w$ are uncorrelated (and thus independent) between scales.

To conclude, we showed that the MRA can be expressed as a multi-resolution autoregressive model, which allows to use a Kalman smoother for inference (Ferreira and Lee, 2007, Ch. 8). Therefore, one can view the MRF as a scale-recursive Kalman smoother nested within each step of an outer Kalman filter, the latter proceeding along the time dimension.

# S4 More details on the numerical simulations in Section 7

## S4.1 Definition of scores

**Kullback-Leibler (KL) divergence** KL divergence is often used as a way of quantifying how different two distributions are. In the context of the simulation study in Section 7, KL divergence measures how much the approximate filtering distribution differs from the exact

distribution calculated by the Kalman filter. Formally, if $f$ is the exact $k$-variate normal distribution with mean $\boldsymbol{\mu}_f$ and covariance matrix $\boldsymbol{\Sigma}_f$, and $g_j$ is the normal distribution obtained using method $j$ with mean $\boldsymbol{\mu}_j$ and covariance $\boldsymbol{\Sigma}_j$, then the KL divergence can be expressed as

$$\mathrm{KL}(f||g_j) = \frac{1}{2}\left(\mathrm{tr}\left(\boldsymbol{\Sigma}_j^{-1}\boldsymbol{\Sigma}_f\right) + \left(\boldsymbol{\mu}_j - \boldsymbol{\mu}_f\right)\boldsymbol{\Sigma}_j^{-1}\left(\boldsymbol{\mu}_j - \boldsymbol{\mu}_f\right) - k + \ln\left(\frac{\det \boldsymbol{\Sigma}_j}{\det \boldsymbol{\Sigma}_f}\right)\right).$$

In Section 7, we have $k = n_{\mathcal{G}} = 1{,}156$. For the KL divergence to be small, we need both the mean and the covariance matrix to be accurate (i.e., $\boldsymbol{\mu}_j \approx \boldsymbol{\mu}_f$ and $\boldsymbol{\Sigma}_j \approx \boldsymbol{\Sigma}_f$).

**Root mean squared prediction error (RMSPE)** MSPE captures how much, on average, the predicted values differ from the true values. In our case, if $\boldsymbol{\mu}_j[i]$ denotes the value predicted by method $j$ (i.e., the filtering mean) of process $\mathbf{x}$ at grid point $i$, and if $\mathbf{x}[i]$ is the true value at this point, RMSPE is calculated as follows:

$$\mathrm{RMSPE} = \sqrt{\frac{1}{n_{\mathcal{G}}}\sum_{i=1}^{n_{\mathcal{G}}}\left(\boldsymbol{\mu}_j[i] - \mathbf{x}[i]\right)^2},$$

where $n_{\mathcal{G}}$ is the number of grid points.

## S4.2 Circular domain

Consider a diffusion-advection model with an initial state drawn from a Gaussian process:

$$\begin{cases} \frac{\partial}{\partial t}x(s,t) = \alpha\frac{\partial}{\partial s}x(s,t) + \beta\frac{\partial^2}{\partial s^2}x(s,t) + \zeta(s,t) \\ x(s,0) \sim GP\left(0, K_{1d}(\cdot,\cdot)\right) \end{cases}. \tag{S5}$$

We assume that $x : S \times [0,T] \to \mathbb{R}$ is the quantity of interest between $t = 0$ and $t = T$, over a one-dimensional sphere with unit circumference, $\zeta$ is a zero-mean stationary Gaussian process with an isotropic spatial covariance function $\sigma_w^2 C(\cdot,\cdot)$ and independent increments over time, and $K_{1d}$ is the spatial covariance function of the process $x$ at time $t = 0$, defined as $K_{1d}(s_1, s_2) = \mathcal{M}_{\nu,\lambda}\left(|s_1 - s_2| \mod 1\right)$.

We discretize both the spatial and the temporal domains using $n_{\mathcal{G}} = 80$ and $T = 20$ regularly spaced points, respectively. Applying first-order forward differences in time and centered differences in space as in Xu and Wikle (2007), we can approximate the derivatives in (S5) with

$$\frac{\partial}{\partial t}x(s,t) \approx \left(x(s,t+\Delta t) - x(s,t)\right)\frac{1}{\Delta t}, \tag{S6}$$

$$\frac{\partial}{\partial s}x(s,t) \approx \left(x(s+\Delta s,t) - x(s-\Delta s,t)\right)\frac{1}{2\Delta s} \tag{S7}$$

$$\frac{\partial^2}{\partial s^2}x(s,t) \approx \left(x(s+\Delta s,t) - 2x(s,t) + x(s-\Delta s,t)\right)\frac{1}{\Delta^2 s}. \tag{S8}$$

Then, taking $\Delta t = 1$ and $\Delta s = \frac{1}{n_{\mathcal{G}}}$, the first equation in (S5) can be expressed as

$$x(s,t) = c_1 \cdot x(s,t-1) + c_2 \cdot x(s+\tfrac{1}{n_{\mathcal{G}}},t-1) + c_3 \cdot x(s-\tfrac{1}{n_{\mathcal{G}}},t-1) \tag{S9}$$

with $c_1 = 1 - 2\beta n_{\mathcal{G}}^2$, $c_2 = 0.5\alpha n_{\mathcal{G}} + \beta n_{\mathcal{G}}^2$ and $c_3 = -0.5\alpha n_{\mathcal{G}} + \beta n_{\mathcal{G}}^2$. Following Xu and Wikle (2007), we use $\alpha = 0.5/n_{\mathcal{G}}, \beta = 0.35/n_{\mathcal{G}}^2$, which correspond to $c_1 = 0.3, c_2 = 0.6, c_3 = 0.1$. These parameters also ensure the stability of the scheme.

The discretization allows us to express the original model (S5) as

$$\begin{cases} \mathbf{x}_t = \mathbf{A}_t \mathbf{x}_{t-1} + \mathbf{w}_t, \\ \mathbf{x}_0 \sim \mathcal{N}(\mathbf{0}, \mathbf{\Sigma}), \end{cases} \tag{S10}$$

where $\mathbf{x}_t$ is a vector with values of $x(\cdot, t)$ at the spatial grid points, the evolution matrix

$$\mathbf{A}_t = \begin{bmatrix} c_1 & c_2 & & & & & c_3 \\ c_3 & c_1 & c_2 & & & & \\ & c_3 & c_1 & c_2 & & & \\ & & & \ddots & & & \\ & & & & c_3 & c_1 & c_2 \\ & & & & & c_3 & c_1 & c_2 \\ c_2 & & & & & & c_3 & c_1 \end{bmatrix} \tag{S11}$$

is tri-diagonal with two non-zero elements in the bottom-left and top-right corners, the covariance matrix

$$\mathbf{\Sigma} = \left[\mathcal{M}_{\nu,\lambda}\left(|s_i - s_j| \mod 2\pi\right)\right]_{i,j=1,\ldots n_{\mathcal{G}}} \tag{S12}$$

is obtained by evaluating $K_{1d}$ at all spatial grid points $s_i$, and $\mathbf{w}_t \sim \mathcal{N}(\mathbf{0}, \sigma_w^2 \mathbf{Q})$ with $\mathbf{Q} = [C(s_i, s_j)]_{i,j=1,\ldots n_{\mathcal{G}}}$. We see that (S10) has the same form as (2) in Section 2.1.

We also assume that at every time point $t$, we have $n_t < n_{\mathcal{G}}$ noisy observations in the vector $\mathbf{y}_t$, each corresponding to a grid point in $\mathcal{G}$. We represent this assumption using (1), where the matrix $\mathbf{H}_t$ is built by removing those rows from $\mathbf{I}_{n_{\mathcal{G}}}$ that correspond to grid points for which no data are available. Thus $\mathbf{H}_t$ is $n_t \times n_{\mathcal{G}}$. Examples of realizations are shown in Figure S2.

## S4.3 Square domain

In the second set of simulations, we consider a rectangular domain, which is common for spatial data sets. We generalize the model (S5) as

$$\begin{cases} \frac{\partial}{\partial t} x(\mathbf{s}, t) = \alpha_1 \frac{\partial}{\partial s_1} x(\mathbf{s}, t) + \alpha_2 \frac{\partial}{\partial s_2} x(\mathbf{s}, t) + \beta \frac{\partial^2}{\partial s_1^2} x(\mathbf{s}, t) + \frac{\partial^2}{\partial s_2^2} x(\mathbf{s}, t)) + \zeta(\mathbf{s}, t) \\ x(\mathbf{s}, 0) = GP\left(0, K_{2d}(\cdot, \cdot)\right) \end{cases} . \tag{S13}$$

We assume that $x(\mathbf{s}, t) : [0, 1]^2 \times [0, T] \to \mathbb{R}$, that $\zeta(\mathbf{s}, t)$ is a two dimensional zero-mean stationary Gaussian process with an isotropic spatial covariance function $\sigma_w^2 C(\cdot, \cdot)$ and independent over time, and we define $K_{2d}(\mathbf{s}_i, \mathbf{s}_j) = \mathcal{M}_{\nu,\lambda}(\|\mathbf{s}_i - \mathbf{s}_j\|_2)$. We set the diffusion coefficient $\beta = 0.0004$ and we use $\alpha_1 = \alpha_2 = 0.01$. Similar to the 1D case, we discretize (S13) using a regular spatial grid with $n_x = n_y = 34$ points along each dimension and 20 equidistant time points. We approximate the time derivative as in Section S4.2 and use the

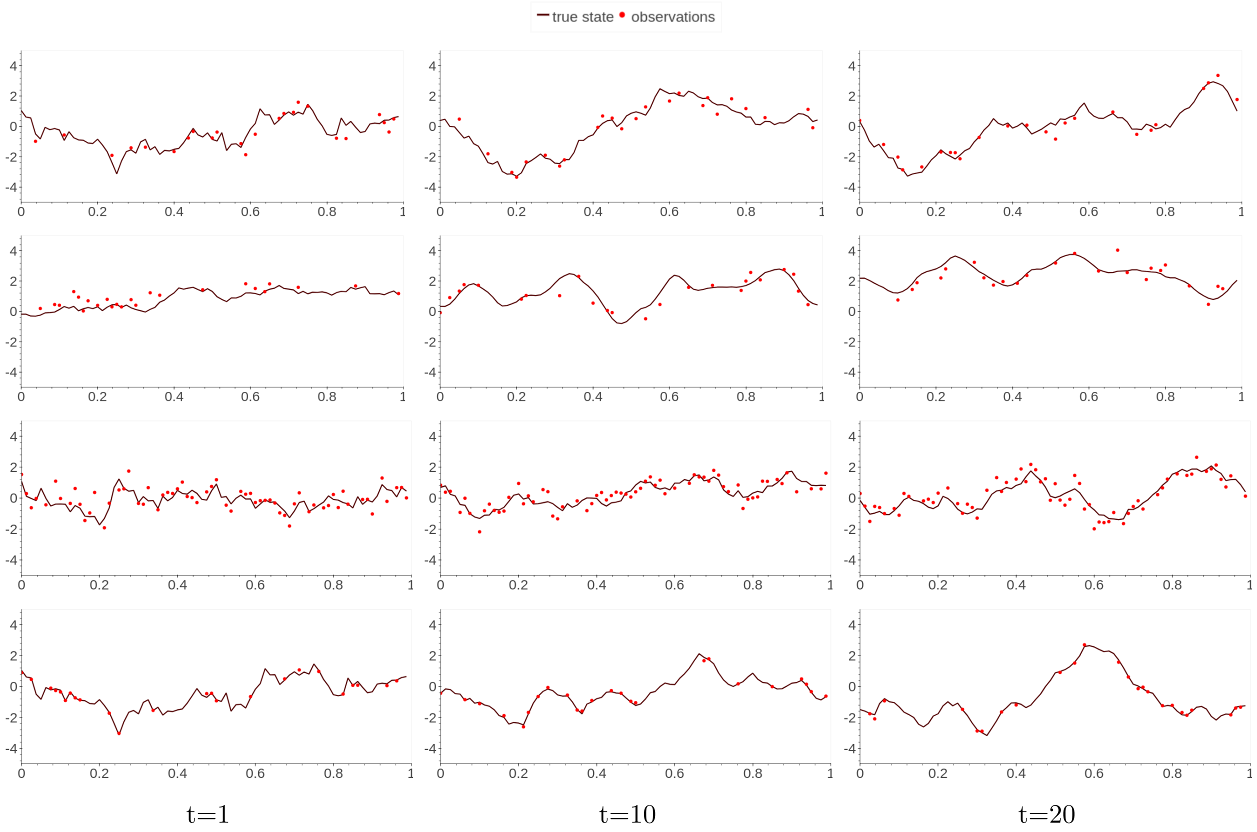


Figure S2: Sample realizations simulated from the model described in Sections 7.1 and S4.2. The rows correspond to the scenarios in Table 1, from top to bottom: baseline, smooth, dense obs., and low noise.

following approximations for the spatial derivatives:

$$\frac{\partial}{\partial \mathbf{s}_1} x(\mathbf{s},t) \approx \left( x(\mathbf{s},t) - x(\mathbf{s} - [\Delta s_1, 0]^T, t) \right) \frac{1}{\Delta s_1}, \tag{S14}$$

$$\frac{\partial}{\partial \mathbf{s}_2} x(\mathbf{s},t) \approx \left( x(\mathbf{s},t) - x(\mathbf{s} - [0, \Delta s_2, ]^T, t) \right) \frac{1}{\Delta s_2}, \tag{S15}$$

$$\frac{\partial^2}{\partial \mathbf{s}_1^2} x(\mathbf{s},t) \approx \left( x(\mathbf{s} - [\Delta s_1, 0]^T, t) - 2x(\mathbf{s}) + x(\mathbf{s} + [\Delta s_1, 0]^T, t) \right) \frac{1}{\Delta^2 s_1}, \tag{S16}$$

$$\frac{\partial^2}{\partial \mathbf{s}_2^2} x(\mathbf{s},t) \approx \left( x(\mathbf{s} - [0, \Delta s_2]^T, t) - 2x(\mathbf{s}) + x(\mathbf{s} + [\Delta s_2, 0]^T, t) \right) \frac{1}{\Delta^2 s_2}. \tag{S17}$$

We set $\Delta s_1 = \Delta s_2 = 1/(n_x + 1) = 0.029$ and $\Delta t = 1$. Similar to the 1D case, we then represent the model (S13) as a linear state-space model:

$$\begin{cases} \mathbf{x}_t = \mathbf{A}_t \mathbf{x}_{t-1} + \mathbf{w}_t, \\ \mathbf{x}_0 \sim \mathcal{N}(\mathbf{0}, \mathbf{\Sigma}), \end{cases} \tag{S18}$$

with the evolution matrix having 5 diagonal nonzero bands. If we use $c_k$ and $c_{-k}$ to denote the values on the $k$-th diagonal above and below the main diagonal, respectively, then all

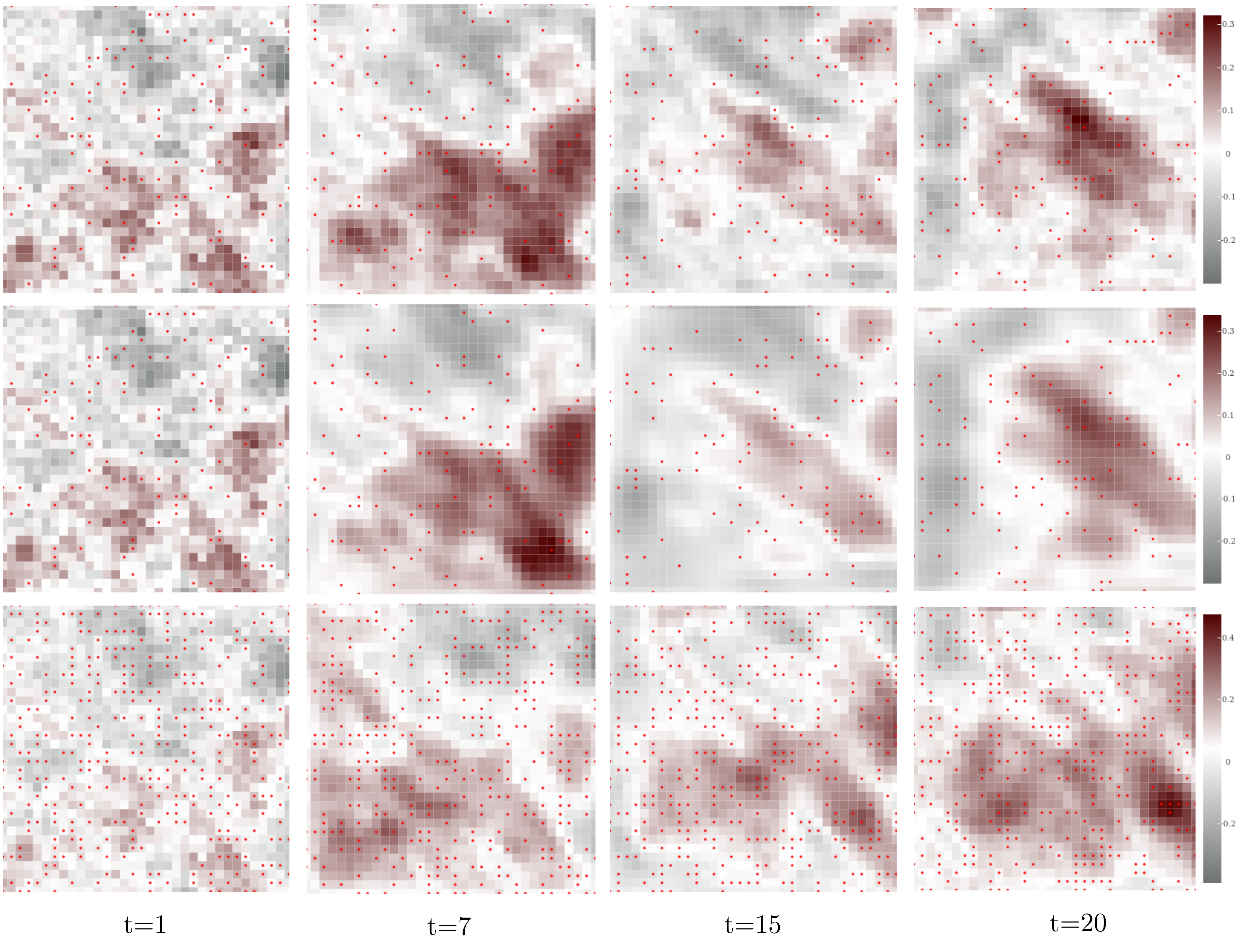


Figure S3: Sample realizations simulated from the model described in Sections 7.2 and S4.3. The rows correspond to the first three scenarios in Table 2, from top to bottom: baseline, smooth, and dense obs. Red dots denote observation locations.

nonzero entries of $\mathbf{A}_t$ are given by:

$$\begin{aligned} c_{-n_x} &= -\beta\Delta^2 s_2 + \alpha_2 \cdot \Delta s_2 \\ c_{-1} &= -\beta\Delta^2 s_1 + \alpha_1 \cdot \Delta s_1 \\ c_0 &= 1 + 2\beta(\Delta^2 s_1 + \Delta^2 s_2) - \alpha_1 \Delta s_1 - \alpha_2 \Delta s_2 \\ c_1 &= -\beta\Delta^2 s_1 \\ c_{n_x} &= -\beta\Delta^2 s_2. \end{aligned}$$

We also take $\mathbf{w}_t \sim \mathcal{N}(\mathbf{0}, \sigma_w^2 \mathbf{Q})$ with $\mathbf{Q} = [C(\mathbf{s}_i, \mathbf{s}_j]_{i,j=1,\dots n_\mathcal{G}}$ and $\mathbf{\Sigma} = [K_{2d}(\mathbf{s}_i, \mathbf{s}_j)]_{i,j=1,\dots n_\mathcal{G}}$. We model the observations in the same way as described in the 1D case. Examples of realizations are given in Figure S3.

## S4.4 Interval coverage

Comparing the frequentist coverage of intervals to their nominal level is a quick way of assessing the calibration of predictive distributions.

Figure S5 presents interval coverage for filtering methods described in Section 7 and using parameter settings discussed there. At each time $t$, we calculate 95% filtering intervals (i.e., with endpoints consisting of the 2.5 and 97.5 percentiles of the filtering distribution) for each grid point and report the proportion of intervals that cover the true value. On average, 95% of exact confidence intervals (i.e., those generated using the Kalman filter) should cover the corresponding true values.

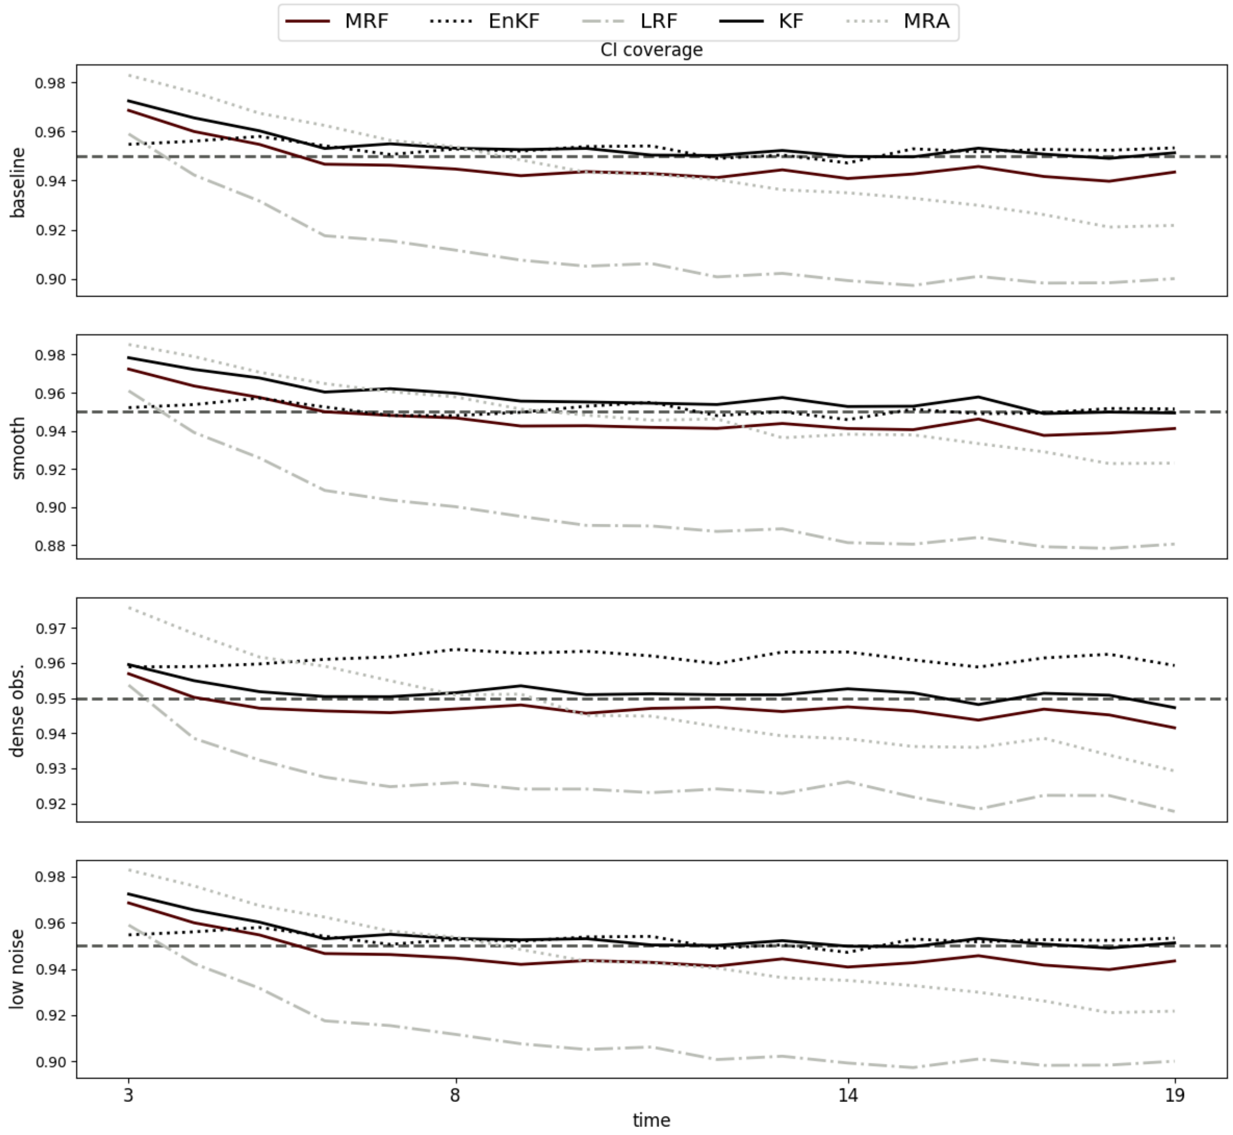


Figure S5: Interval coverage for different filtering methods. Straight dashed horizontal line indicates the nominal coverage (95%).

The interval coverage is similar to the nominal coverage under all parameter settings for Kalman filter, EnKF, and MRF. The filtering distributions of the remaining two methods seem to be poorly calibrated: low-rank filter generates intervals that are too narrow, while the ones produced by MRA start as too wide and become too narrow as time progresses.

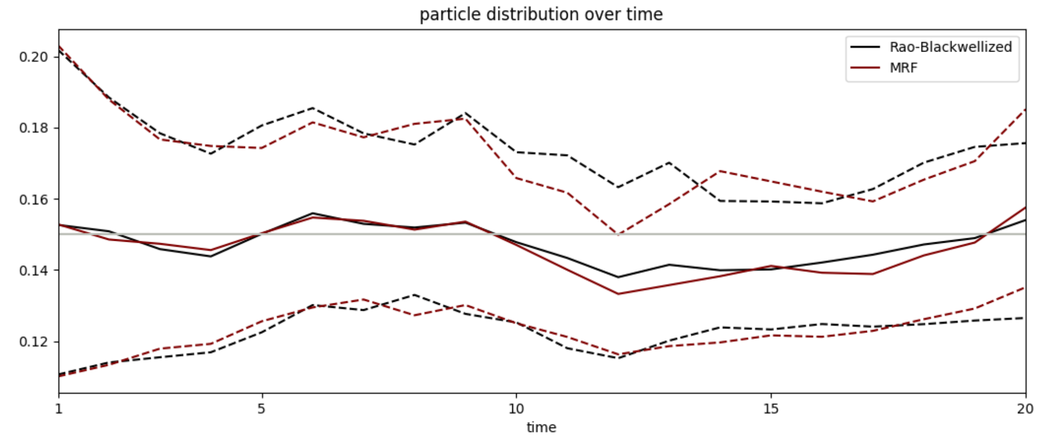


Figure S6: Summary of particle distributions over time. The solid line is the mean and the dashed lines are the 10th and 90th percentiles, respectively, of the filtering distributions. The solid grey line indicates the true value of the parameter.

Table S1: Root mean squared error of MLEs of the range parameter $\lambda$, as implied by three different integrated likelihoods

| | exact | MRF | LRF |
|---|---|---|---|
| RMSE | 0.057 | 0.066 | 0.076 |

# S5 Numerical experiments using the particle MRF

In order to illustrate the performance of the particle MRF described in Section 6, we simulated data from the two-dimensional model with baseline parameter settings (see Sections 7 and S4.3), and used Algorithm 3 to infer the filtering distribution of a $\lambda$, the range parameter of the innovation covariance matrix. We assumed the prior distribution to be such that $\log \lambda_t \sim N(\log(0.15), 0.25^2)$. The proposal distribution was taken to be $\log \lambda_t | \lambda_{t-1} \sim N(\log \lambda_{t-1}, 0.5^2)$, while the initial values were drawn from $\log \lambda_0 \sim N(\log(0.15), 0.25^2)$. Figure S6 shows the performance of the MRF and the exact Rao-Blackwellized (Doucet et al., 2000) particle filters, both using 1,000 particles. The particle MRF produced similar distributions as the exact filter.

We also compared the accuracy of parameter inference using the MRF to that using the LRF, which can be viewed as a special case of the MRF as described in Section 7. We simulated 50 datasets at a single time point $t = 1$, assuming the 2D baseline settings, except that $x_0$ and $\mathbf{\Sigma}_{0|0}$ were initialized as zero. For each dataset and each method, we numerically found the $\lambda$ value that maximized the integrated likelihood $\mathcal{L}_t$ from (6) at time $t = 1$. The distributions of the resulting 50 parameter estimates are summarized in Figure S7, while Table S1 contains the root mean squared error of the MLEs for each of the methods.

While both approximate methods produced acceptable results, the estimates obtained by the MRF were considerably more accurate than those produced by the LRF, both at the same computational complexity.

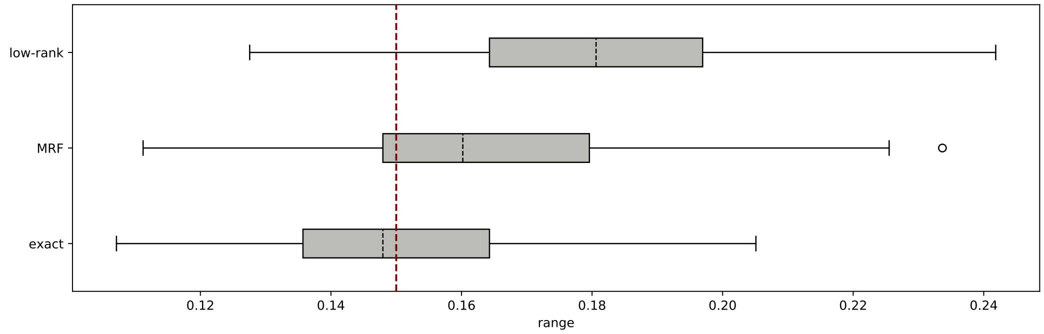


Figure S7: Boxplots of MLEs of the range parameter $\lambda$, as implied by three different integrated likelihoods. The true value $\lambda = 0.15$ is indicated by the vertical dashed line.

# S6 Review of some graph theoretical results

In this section we define several terms commonly used in graph theory that will be needed in Section S8. These definitions follow the terminology used in Lauritzen (1996) and Khare and Rajaratnam (2012). We denote by $G(V, E)$ a graph with vertices $V$ and edges $E$.

Definition S2. *We call $G'$ a* subgraph *induced by $A \subseteq V$ if $G' = (A, E \cap (A \times A))$.*

In other words, a subgraph is a graph formed by taking a subset $A$ of vertices and all the edges whose endpoints are in $A$.

Definition S3. *A* path *is a sequence of vertices $v_1, \dots, v_n \subset V$ such that for $i = 1, \dots, n$, $(v_i, v_{i-1}) \in E$. A* cycle *is a path such that $v_n = v_1$.*

Definition S4. *Consider a* cycle *$(v_1, \dots, v_n)$. A chord is an edge $e \in E$ which connects two non-consecutive vertices within the cycle. Graph $G$ is* chordal *if every cycle of length greater than 4 has a chord.*

Chordal graphs are also called triangulated graphs or decomposable graphs.

Definition S5. *A graph is* homogeneous *if it is chordal and if it does not contain the graph $A_4$, defined as $\overset{1}{\bullet} - \overset{2}{\bullet} - \overset{3}{\bullet} - \overset{4}{\bullet}$, as an induced subgraph.*

Following Khare and Rajaratnam (2012), we write that $v \to w$ when

$$\{u : u = w \vee (u, w) \in E\} \subseteq \{u : u = v \vee (u, v) \in E\}. \tag{S19}$$

In other words, when $v \to w$, then the neighborhood (all direct neighbors) of $w$ is contained within the neighborhood of $v$. Within the context of of our graph $G$, we can make the symbol $\to$ more intuitive by thinking of if it as saying that "$w$ is downstream from $v$." In principle, it is possible that two vertices have the exact same neighborhoods. To capture it formally, we could define an equivalence relation $\equiv$ as

$$u \equiv v \iff u \to v \,\wedge\, v \to u.$$

We denote by $\bar{v}$ the equivalence class under $\equiv$ containing $v$.

Definition S6. *For a homogeneous graph $G = (V, E)$, an ordering $\sigma$ is called a* Hasse tree-based elimination scheme *for $G$, if for $u, v \in V$*

$$u \to v, \bar{u} \neq \bar{v} \implies \sigma(u) > \sigma(v),$$

which we adopt after Khare and Rajaratnam (2012).

Definition S7. *A* tree *is a directed graph with no cycles, such that each vertex has degree one (i.e., for a vertex $u$, there is only one edge that ends at $u$).*

Definition S8. *Let $T = (V, E)$ be a tree and let $(i, j) \in E$. Then $i$ is called a* parent *of $j$, while $j$ is called a* child *of $i$.*

# S7 Hierarchical matrices

This section introduces basic concepts of hierarchical matrix theory. They come in useful in the proof of Lemma S1 in Section S8.

If $t$ is a vertex of a tree $T$, let $c(t)$ denote the set of children of $t$. Formally, $c(t) := \{s \in T : s \text{ is a child of } t\}$. Similarly, if $s \in c(t)$ (i.e., $t$ is a parent of $s$), we write $t = p(s)$.

Definition S9. (Hackbusch, 1999) *Let $I$ be an index set. A tree $T$ is called an $\mathcal{H}$-*tree *(based on $I$) if the following conditions hold:*

1. *All vertices $t \in T$ are subsets of $I$;*
2. *$I \in T$;*
3. *$|c(t)| \neq 1 \quad \forall t \in T$.*

It can be concluded that $I$ is the root of $T$, the only vertex without a parent element.

Definition S10. *The* depth *of a vertex $t$ is a function $d(\cdot)$ defined as*

$$d(t) = \begin{cases} 0 & \textit{if } t \textit{ is the root} \\ d(p(t) + 1) & \textit{otherwise} \end{cases}. \tag{S20}$$

Our notation will often be more readable if we write $t \searrow s$ whenever $d(t) > d(s)$, and $t \nearrow s$ if $d(t) < d(s)$.

We use $\mathcal{A}(t)$ to label the set of all ancestors of the vertex $t$, that is

$$\mathcal{A}(s) = \begin{cases} \emptyset & \text{if t is the root} \\ \mathcal{A}(p(s)) \cup \{p(s)\} & \text{otherwise} \end{cases}. \tag{S21}$$

Throughout Section S8 and Appendix A, we assume for simplicity that $r = 1$. If this is not true, we can consider an equivalence relation $\equiv_m$ such that for two columns $\mathbf{c}_1, \mathbf{c}_2$ in $\mathbf{B}^m$ $\mathbf{c}_1 \equiv_m \mathbf{c}_2 \iff \mathbf{c}_1, \mathbf{c}_2$ both contain elements of the same block $\mathbf{B}_{j_1,\ldots,j_m}$. Verification that $\equiv_m$ is indeed an equivalence relation is elementary. The assumption that $r = 1$ means that each of the blocks $\mathbf{B}_{j_1,\ldots,j_m}$ has dimensions $|\mathcal{I}_{j_1,\ldots,j_m}| \times 1$.

Now notice that the partitioning scheme defined in Section 3.4.1 is an $\mathcal{H}$-tree based on $\mathcal{I}$. Indeed: (1) all elements $\mathcal{I}_{j_1,\ldots,j_m}$ are subsets of $\mathcal{I}$, (2) $\mathcal{I}$ is the root node and (3) $|c(\mathcal{I}_{j_1,\ldots,j_m})| = J > 1$. We will refer to this $\mathcal{H}$-tree as $T_\mathcal{I}$. From this perspective, each $\mathcal{I}_{j_1,\ldots,j_m}$ is a vertex of $T_\mathcal{I}$. Figure S8a illustrates $T_\mathcal{I}$ for the case $M = 3$ and $J = 2$.

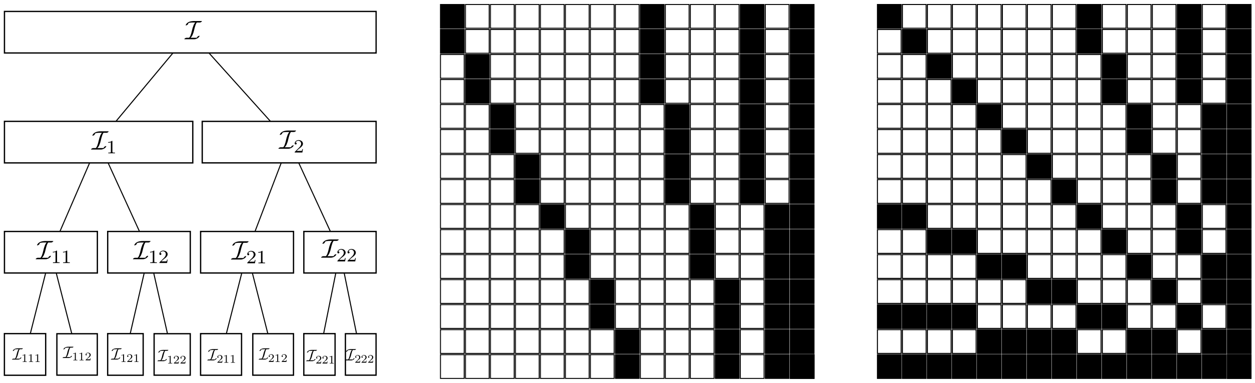


(a) An $\mathcal{H}$-tree over grid $\mathcal{I}$ (b) $\mathbf{B}$ matrix (c) $\mathbf{B}'\mathbf{B}$ matrix

Figure S8: Mapping $\tau$ used in Section S8 goes from b) to a), while mapping $\pi$ goes from b) to c).

# S8 Lemmas used in the proof of Proposition 3

Lemma S1. *The pattern of zeros in* $\mathbf{B}'\mathbf{B}$ *corresponds to a homogeneous graph.*

*Proof.* We start by observing that there is a $1-1$ mapping $\tau : \mathcal{I} \to T_{\mathcal{I}}$ between the indices of columns of $\mathbf{B}$ and the vertices of $T_{\mathcal{I}}$. Specifically, each index $j \in \mathcal{I}$ of some column $\mathbf{c}_j$ can be identified with the vertex that has the same index as the $\mathbf{B}_{j_1,\ldots,j_m}$ block that $\mathbf{c}_j$ contains. For example, by construction, $\mathbf{c}_1$, the first column in $\mathbf{B}^M$, contains elements $\mathbf{B}_{1,\ldots,1}$, so $\tau(1) = \mathcal{I}_{1,\ldots,1}$. Also notice that if $\mathbf{c}_i$ contains $\mathbf{B}_{j_1,\ldots,j_m}$ and $\mathbf{c}_j$ contains $\mathbf{B}_{j_1,\ldots,j_{m-1}}$, then $\tau(j) \in \mathcal{A}(\tau(i))$ (see Figure S8 for illustration).

Next, take two columns $\mathbf{c}_i, \mathbf{c}_j$ of $\mathbf{B}$ and $\tau(i), \tau(j)$, the corresponding vertices in $T_{\mathcal{I}}$. For the rest of the proof, we assume without loss of generality that $i < j$. Then there are two cases to consider.

1. $d(\tau(i)) = d(\tau(j))$:
   In this situation $\mathbf{c}_i'\mathbf{c}_j = 0$ because $\mathbf{c}_i, \mathbf{c}_j$ are columns of the same block diagonal matrix $\mathbf{B}^m$ and each diagonal block is only one column wide.

2. $d(\tau(i)) > d(\tau(j))$:
   We examine two subcases:

   (a) $\tau(j) \notin \mathcal{A}(\tau(i))$; this implies that $\mathbf{c}_i'\mathbf{c}_j = 0$;

   (b) $\tau(j) \in \mathcal{A}(\tau(i))$; then, in general, $\mathbf{c}_i'\mathbf{c}_j \neq 0$.

Let us now look at $\mathbf{B}'\mathbf{B}$ as an adjacency matrix of graph $G = (\mathcal{I}, E)$ where

$$E = \{(i,j) : \mathbf{B}'\mathbf{B}_{ij} \neq 0\}.$$

Define $\pi$ as a mapping that assigns a vertex in $G$ to each column of $\mathbf{B}$, i.e. $\pi(\mathbf{c}_j) = j$ for each $j \in \mathcal{I}$. Defining $\rho := \tau \circ \pi^{-1}$ gives us a $1-1$ correspondence between the vertices of graph $G$ and $T_{\mathcal{I}}$ (Figure S8). We can thus define $d$, $\mathcal{A}$, $c$ and $p$ for the vertices of the undirected graph $G$ by referring to the corresponding definitions on $T_{\mathcal{I}}$. For example, if $u$ is some vertex of $G$, then $\mathcal{A}(u) := \mathcal{A}(\rho(u))$.

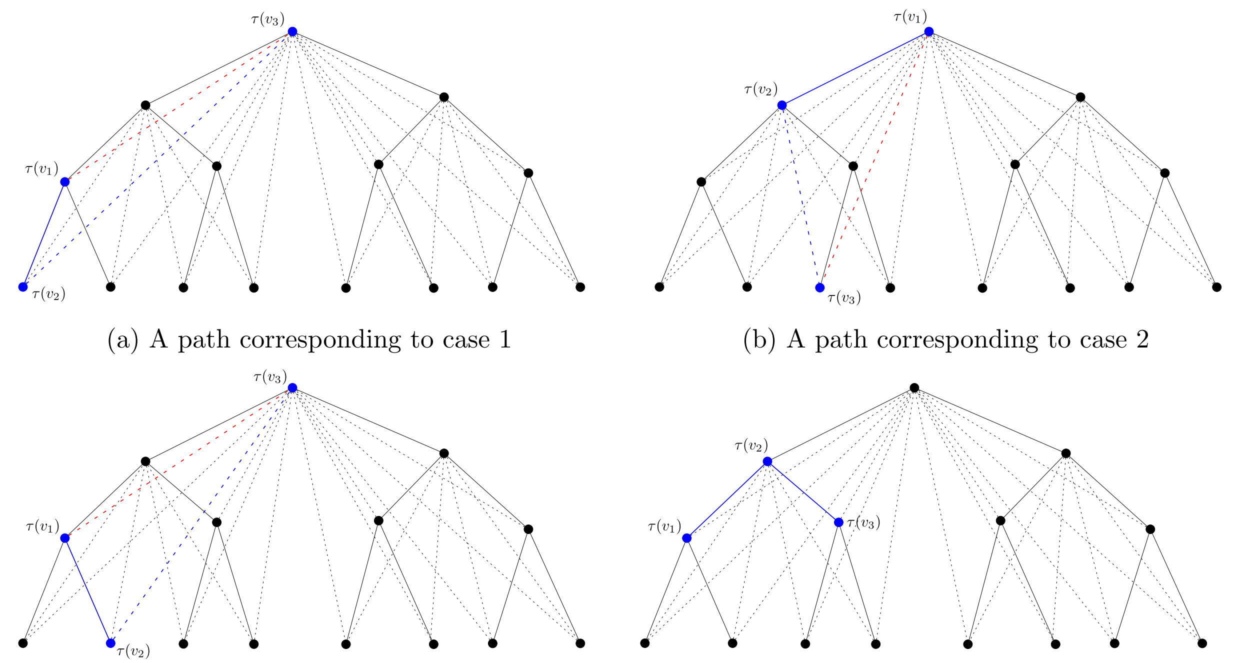


(a) A path corresponding to case 1

(b) A path corresponding to case 2

(c) A path corresponding to case 3

(d) A path corresponding to case 4

Figure S9: Different paths of length 3 in graph G considered in the proof of Lemma S1. For clarity, dashed lines were used to indicate edges that connect vertices whose depths differ by more than 1. Elements of the path are marked in blue. A red line indicates a chord.

Using this new notation, the fact that $\mathbf{B}'\mathbf{B}_{ij} = \mathbf{c}_i'\mathbf{c}_j$, as well as the previous observations, we have

$$(i, j) \in E \iff i \in \mathcal{A}(j). \tag{S22}$$

In particular, if $d(i) = d(j)$ then $(i, j) \notin E$.

Next, let $(v_1, v_2, v_3, v_4)$ be some path in $G$. We will show that each such path contains a chord, which means that either $(v_1, v_3) \in E$ or $(v_2, v_4) \in E$. There are four cases we need to consider to demonstrate this (see Figure S9):

1. $v_1 \nearrow v_2 \nearrow v_3$:
   This means that $v_3 \in \mathcal{A}(v_1)$, and so $(v_3, v_1) \in E$ is a chord.

2. $v_1 \searrow v_2 \searrow v_3$:
   In this case $v_1 \in \mathcal{A}(v_3)$, and so $(v_3, v_1) \in E$ is a chord.

3. $v_1 \searrow v_2 \nearrow v_3$:
   Let $d(v_3) < d(v_1)$. Then $v_3$ has to be a descendant of $v_1$, and so $(v_3, v_1) \in E$ is a chord. If $d(v_3) > d(v_1)$, then $v_1$ is a descendant of $v_3$. It is not possible that $d(v_1) = d(v_3)$ and $v_3 \neq v_1$, because every node has only one parent.

4. $v_1 \nearrow v_2 \searrow v_3$:
   We need to consider two subcases here:

   (a) $v_3 \searrow v_4$; this means that $v_2 \searrow v_3 \searrow v_4$, which reduces to case 2;

(b) $v_3 \nearrow v_4$; this means that $v_2 \searrow v_3 \nearrow v_4$, which reduces to case 3.

The reasoning above shows that $A_4$ is not a subgraph of G and that G is decomposable. Therefore we conclude that $G$ is homogeneous. □

LEMMA S2. *Let $G = (\mathcal{I}, E)$ be the graph described by the pattern of zeros in our $\mathbf{B}'\mathbf{B}$ matrix. Let $\sigma$ be an ordering of the vertices of $G$ such that*

$$\sigma(i) = i.$$

*Then $\sigma$ is a Hasse tree based elimination scheme for $G$.*

*Proof.* Let $N(u) = \{v \in G : (v, u) \in E\} \cup \{u\}$.

We begin by showing that

$$N(v) \subsetneq N(u) \iff u \in \mathcal{A}(v). \tag{S23}$$

First, let us assume that $u \in \mathcal{A}(v)$, and take some $w$ such that $u \in \mathcal{A}(w)$ and $w \in \mathcal{A}(v)$. Because $u$ is not a leaf, Definition S9 implies $|S(u)| > 1$. Therefore, there exists a $w' \neq w \in S(u)$. Since $w' \notin \mathcal{A}(v)$, by (S22) $w'$ is not a neighbor of $v$, but it is a neighbor of $u$. Now observe that

$$N(v) = \mathcal{A}(v) \cup \{v\} \cup \{w : v \in \mathcal{A}(w)\}.$$

Let $w \in \{v\} \cup \{w : v \in \mathcal{A}(w)\}$, then we have $v \in \mathcal{A}(w)$. Thus $w \in N(v)$. Now take $w \in \mathcal{A}(v)$. We have three cases here:

- if $d(w) < d(v)$, then $v \in \mathcal{A}(w)$ and so $w \in N(v)$;
- if $d(w) = d(v)$, then $w = v$ and so $w \in N(v)$;
- if $d(w) > d(v)$, then $w \in \mathcal{A}(v)$ and so $w \in N(v)$.

Thus we showed that $N(v) \subset N(u)$ but $N(v) \neq N(u)$.

Second, assuming $N(v) \subsetneq N(u)$ implies that $(v, u) \in \mathcal{E}$, so either $v \in \mathcal{A}(u)$ or $u \in \mathcal{A}(v)$. But if the former was to hold, it would contradict what we have shown above. Therefore, we conclude that $u \in \mathcal{A}(v)$.

The equivalence we have just demonstrated means that the lemma is proved once we show that

$$u \in \mathcal{A}(v) \implies \sigma(u) > \sigma(v).$$

But we already established in (S22) that

$$\begin{cases} i < j \\ (i, j) \in E \end{cases} \iff i \in \mathcal{A}(j). \tag{S24}$$

This means that if we order the vertices in $V$ according to the order of the rows of $\mathbf{B}'\mathbf{B}$ to which they correspond, this ordering will be a Hasse tree-based elimination scheme. □

## References

Choi, M. J., Chandrasekaran, V., and Willsky, A. S. (2010). Gaussian multiresolution models: Exploiting sparse markov and covariance structure. *IEEE Transactions on Signal Processing*, 58(3):1012–1024.

Chou, K. C., Willsky, A. S., and Benveniste, A. (1994a). Multiscale recursive estimation, data fusion, and regularization. *IEEE Transactions on Automatic Control*, 39(3):464–478.

Chou, K. C., Willsky, A. S., and Nikoukhah, R. (1994b). Multiscale systems, Kalman filters, and Riccati equations. *IEEE Transactions on Automatic Control*, 39(3):479–492.

Doucet, A., de Freitas, N., Murphy, K., and Russell, S. (2000). Rao-Blackwellised particle filtering for dynamic Bayesian networks. *Proceedings of the Sixteenth Conference on Uncertainty in Artificial Intelligence*, pages 176–183.

Ferreira, M. A. and Lee, H. K. (2007). *Multiscale Modeling: A Bayesian Perspective*. Springer Science & Business Media.

Frakt, A. B. and Willsky, A. S. (2001). Computationally efficient stochastic realization for internal multiscale autoregressive models. *Multidimensional Systems and Signal Processing*, 12(2):109–142.

Hackbusch, W. (1999). A sparse matrix arithmetic based on H-matrices. Part I: Introduction to H-matrices. *Computing*, 62(2):89–108.

Huang, H.-C., Cressie, N., and Gabrosek, J. (2002). Fast, resolution-consistent spatial prediction of global processes from satellite data. *Journal of Computational and Graphical Statistics*, 11(1):63–88.

Johannesson, G., Cressie, N., and Huang, H.-C. (2003). Dynamic multi-resolution spatial models. In Higuchi, T., Iba, Y., and Ishiguro, M., editors, *Proceedings of AIC2003: Science of Modeling*, volume 14, pages 167–174, Tokyo. Institute of Statistical Mathematics.

Katzfuss, M. (2017). A multi-resolution approximation for massive spatial datasets. *Journal of the American Statistical Association*, 112(517):201–214.

Khare, K. and Rajaratnam, B. (2012). Sparse matrix decompositions and graph characterizations. *Linear Algebra and its Applications*, 437(3):932–947.

Lauritzen, S. L. (1996). *Graphical models*, volume 17. Clarendon Press.

Luettgen, M. R. and Willsky, A. S. (1995). Likelihood calculation for a class of multiscale stochastic models, with application to texture discrimination. *IEEE transactions on image processing*, 4(2):194–207.

Tzeng, S., Huang, H.-C., and Cressie, N. (2005). A fast, optimal spatial-prediction method for massive datasets. *Journal of the American Statistical Association*, 100(472):1343–1357.

Willsky, A. S. (2002). Multiresolution markov models for signal and image processing. *Proceedings of the IEEE*, 90(8):1396–1458.

Xu, K. and Wikle, C. K. (2007). Estimation of parameterized spatio-temporal dynamic models. *Journal of Statistical Planning and Inference*, 137(2):567–588.
